# Supplementary material for: Unstable and stable regimes of polariton condensation
Source: arXiv:1707.05798 ancillary file (2018-03-29)
Supplement: Supplementary file 1 [file Supplementary_Material.pdf]

# Supplemental Material for:
# "Unstable and stable regimes of polariton condensation"

F. Baboux,[1,2] D. De Bernardis,[3,4,5] V. Goblot,[1] V.N. Gladilin,[3] C. Gomez,[1] E. Galopin,[1] L. Le Gratiet,[1] A. Lemaître,[1] I. Sagnes,[1] I. Carusotto,[4] M. Wouters,[3] A. Amo,[1] and J. Bloch[1]

[1] *Centre de Nanosciences et de Nanotechnologies, CNRS, Univ. Paris-Sud, Université Paris-Saclay, C2N–Marcoussis, F-91460 Marcoussis, France*

[2] *Laboratoire Matériaux et Phéenomènes Quantiques, Université Paris Diderot, CNRS-UMR 7162, Paris 75013, France*

[3] *TQC, Universiteit Antwerpen, Universiteitsplein 1, B-2610 Antwerpen, Belgium*

[4] *INO-CNR BEC Center and Dipartimento di Fisica, Università di Trento, I-38123 Povo, Italy*

[5] *Vienna Center for Quantum Science and Technology, Atominstitut, TU Wien, 1040 Vienna, Austria*

**Contents**

I. Theory 1

A. Parameters used in the model and numerical methods 1

B. Linear stability analysis 3

C. Temporal dynamics of the instability 4

D. Relation between coherence time and polariton decay rate 5

E. Effect of disorder on the coherence properties 6

II. Experiment 8

A. Determination of the polariton linewidth 8

B. Spatio-temporal behavior of the coherence 8

References 9

## I. Theory

### A. Parameters used in the model and numerical methods

We first give the values of the parameters entering in Eqs. (1)-(2) of the article, and used for our numerical simulations (both in the main text and in this Supplemental Material). The polariton mass $|m| \simeq 5 \times 10^{-5}\, m_0$ is extracted from the measured polariton dispersion. The polariton linewidth is extracted from the low-power photoluminescence in the far field, as detailed in Section II A below: a linear parametrization $\gamma(k) = \gamma_0 + \gamma'|k|$ fairly reproduces the experimental data, with $\hbar\gamma_0 = 90\,(170)$ $\mu$eV for the high (moderate) $Q$ wire cavities, $\hbar\gamma_0 = 75\,(130)$ $\mu$eV for the high (moderate) $Q$ lattices, and $\gamma'/\gamma_0 = 0.7\,(1.6)$ $\mu$m for the wires (lattices) of both quality factors. The reservoir decay

rate is set to $\hbar\gamma_R = 2$ $\mu$eV (corresponding to a lifetime of $\simeq 300$ ps) in agreement with previous measurements of the reservoir lifetime in GaAs cavities [1, 2]. The ratio $g_R/\hbar R \simeq 1$ between the polariton-reservoir interaction constant and the reservoir relaxation rate is determined from the excitonic blueshift $E_x$ at threshold power (through $E_x = 2g_R\gamma/R$), and the polariton-polariton interaction constant $g = X^2 g_R \simeq 0.2\, g_R$ is deduced from the excitonic Hopfield coefficient $X \simeq 0.45$ of the polariton wavefunction for the considered detuning ($\delta \simeq -10$ meV). The pump intensity is set to $P = 2P_{\text{th}}$ (where $P_{\text{th}} = \gamma\gamma_R/R$) for the simulations in the wire cavities and $P = 1.3P_{\text{th}}$ in the lattices.

For the simulations of the condensate density and spatio-temporal coherence reported in Fig. 1 and 2 of the article, we took into account the finite size of the pump spot (Gaussian with 90 $\mu$m FWHM), the presence of a disorder potential $V_{\text{dis}}$, and a dynamical noise term $\mathcal{F}$ accounting for quantum, thermal and pump fluctuations. We thus solved the following equations for the coupled polariton/reservoir dynamics:

$$\begin{cases} i\hbar\frac{\partial\psi}{\partial t} = \left[-\frac{\hbar^2\Delta}{2m} + V_{\text{dis}} + g\,|\psi|^2 + 2g_R n_R + \frac{i\hbar}{2}\left(Rn_R - \gamma\right)\right]\psi + \mathcal{F} & \text{(S1)} \\ \frac{\partial n_R}{\partial t} = P(\mathbf{r}) - (\gamma_R + R\,|\psi|^2)n_R & \text{(S2)} \end{cases}$$

For the simulations in the lattice, we followed Ref. [3] to discretize these equations within the tight-binding approximation.

The disorder potential $V_{\text{dis}}$ is chosen with a standard deviation of the order of 30 $\mu$eV corresponding to the typical disorder strength of our cavities [4]; examples of numerical disorder landscapes are shown in Fig. S1. The dynamical noise is taken to be spatially and temporally uncorrelated:

$$\langle \mathcal{F}(t,x)\mathcal{F}(t',x')\rangle\, dt = F^2 \delta_{t,t'}\delta_{x,x'} \tag{S3}$$

with an amplitude $F$ adjusted to fit the experimentally measured coherence time.

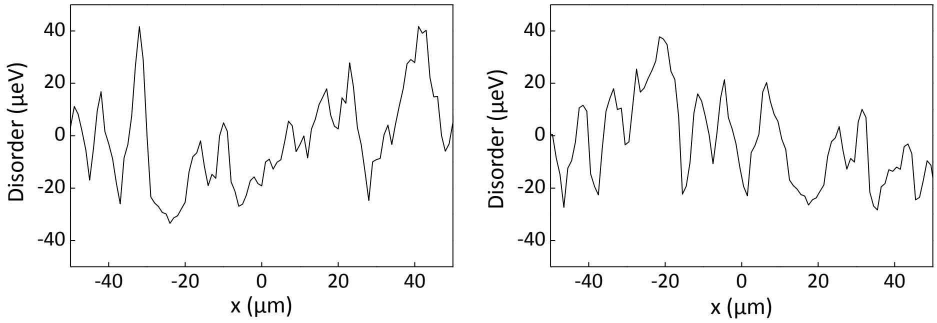


FIG. S1. Examples of numerical disorder landscapes used for the simulations.

The evolution of the condensate wavefunction $\psi$ and reservoir density $n_R$ are calculated by using the split-step algorithm and the Runge-Kutta algorithm, respectively. The time averaged polariton density is then calculated as:

$$\langle|\psi(x)|^2\rangle = \lim_{T\to\infty}\frac{1}{T}\int_0^T |\psi(t,x)|^2 dt \tag{S4}$$

and the time averaged spatio-temporal coherence is obtained as:

$$g^{(1)}(x,-x,t)=\lim_{T\to\infty}\frac{\int_0^T \psi^*(x,t')\psi(-x,t'+t)dt'}{\sqrt{\langle|\psi(x)|^2\rangle\,\langle|\psi(-x)|^2\rangle}} \tag{S5}$$

Finally, we note that for simulations under the adiabatic approximation (see e.g. section I C below), the set of coupled Eqs. (S1)-(S2) reduces to a single equation:

$$i\hbar\frac{\partial\psi}{\partial t}=\left[-\frac{\hbar^2\Delta}{2m}+V_{\text{dis}}+g\,|\psi|^2+\frac{2g_R P}{\gamma_R+R\,|\psi|^2}+\frac{i\hbar}{2}\left(\frac{RP}{\gamma_R+R\,|\psi|^2}-\gamma\right)\right]\psi+\mathcal{F} \tag{S6}$$

### B. Linear stability analysis

We here give the theoretical background for the calculation of the excitation spectra shown in Fig. 3 of the article. We assume a translationally invariant system (homogeneously pumped, and without disorder) and we perform a linear stability analysis in terms of Bogoliubov excitations [5], as follows.

Above the condensation threshold $P>P_{\text{th}}=\gamma\gamma_R/R$, the steady-state solution is a condensate of homogeneous density $|\psi_0|^2=\frac{\gamma_R}{R}(\frac{P}{P_{th}}-1)$ coupled to an homogeneous reservoir density $n_R^0=\frac{\gamma}{R}$. To calculate the response to small perturbations around this steady-state solution, we introduce in the system of equations (1)-(2) of the main text, the following ansatz:

$$\psi(t,x)=\psi_0 e^{-i(\mu_T/\hbar)t}\,(1+\delta\psi(t,x)) \tag{S7}$$

$$n(t,x)=n_R^0\,(1+\delta n_R(t,x)) \tag{S8}$$

where $\mu_T=g|\psi_0|^2+2g_R n_R^0$ plays a role analogous to the chemical potential of equilibrium systems. As previously discussed, we assume the linewidth to depend on $k$ as $\gamma(k)=\gamma_0+\gamma'|k|$. Keeping only terms to first order in $\delta\psi$ and $\delta n_R$, and Fourier transforming the spatial coordinate we obtain the motion equations in a matricial form:

$$i\hbar\partial_t\begin{pmatrix}\delta\psi(t,k)\\ \delta\psi^*(t,k)\\ \delta n_R(t,k)\end{pmatrix}=\begin{pmatrix}\frac{\hbar^2k^2}{2m}-i\hbar\gamma'|k|+g|\psi_0|^2 & g|\psi_0|^2 & 2g_Rn_R^0+\frac{i\hbar}{2}Rn_R^0\\ -g|\psi_0|^2 & -\frac{\hbar^2k^2}{2m}-i\hbar\gamma'|k|-g|\psi_0|^2 & -2g_Rn_R^0+\frac{i\hbar}{2}Rn_R^0\\ -i\hbar R|\psi_0|^2 & -i\hbar R|\psi_0|^2 & -i\hbar(R|\psi_0|^2+\gamma_R)\end{pmatrix}\begin{pmatrix}\delta\psi(t,k)\\ \delta\psi^*(t,k)\\ \delta n_R(t,k)\end{pmatrix} \tag{S9}$$

The spectrum $\omega(k)$ of the matrix corresponds to the spectrum of the elementary (Bogoliubov) excitations of the system, and information about the stability is contained in the imaginary part. The stability of the steady-state solution requires that $\text{Im}[\omega(k)]<0$ for all $k$ (see e.g. Fig. 3f of the article) so that any perturbation is exponentially damped by the system. If on the contrary $\text{Im}[\omega(k)]>0$ in a given region of momentum space (see e.g. Fig. 3c,d,e), the corresponding perturbations will be exponentially amplified, corresponding to an unstable regime. Note that the instability of the linear analysis of the homogeneous system is a necessary condition for the instability in the non-homogeneous system [6].

For the linear stability analysis in the adiabatic approximation (see e.g. Fig. 3a,b of the article), the equation system (S9) has to be replaced with:

$$i\hbar\partial_t\begin{pmatrix}\delta\psi(t,k)\\ \delta\psi^*(t,k)\end{pmatrix}=\begin{pmatrix}\frac{\hbar^2k^2}{2m}+g_{\text{eff}}|\psi_0|^2-\frac{i\hbar\Gamma}{2} & g_{\text{eff}}|\psi_0|^2-\frac{i\hbar\Gamma}{2}\\ -g_{\text{eff}}|\psi_0|^2-\frac{i\hbar\Gamma}{2} & -\frac{\hbar^2k^2}{2m}-g_{\text{eff}}|\psi_0|^2-\frac{i\hbar\Gamma}{2}\end{pmatrix}\begin{pmatrix}\delta\psi(t,k)\\ \delta\psi^*(t,k)\end{pmatrix} \tag{S10}$$

where $\Gamma = \gamma\left(1 - \frac{P_{\rm th}}{P}\right)$.

### C. Temporal dynamics of the instability

In this section we present simulations of the time evolution of the condensate and reservoir, so as to provide some intuitive insights into the physics of the polariton instability. As in the section above, for pedagogical purposes we consider the simplest case of an homogeneously pumped system, without disorder and noise. We use the parameters corresponding to the moderate $Q$ wire cavity (see section I A)

As seen in Fig. S2a (which will be described in greater details below), the unstable dynamics is characterized by the spontaneous creation and propagation of density and phase defects (caused by the hole-burning effect), without the possibility to relax to a stable steady state. The long time dynamics remains turbulent and, under certain assumptions, it is possible to prove that it is affected by spatio-temporal chaos [7–9]. This spatio-temporal chaos is responsible for the short spatio-temporal coherence, even if the system is fully deterministic and not affected by noise. Similar phenomena were studied in the context of pattern formation in non-linear partial differential equations, such as the Ginzburg-Landau equation, which plays an important role in the physics of superconductivity and superfluidity [9].

Figure S2a,b shows the simulated time evolution of the condensate density $|\psi|^2$ and exciton reservoir density $n_R$, respectively, under the adiabatic approximation. The time is given in units of the polariton lifetime $\tau_p = 1/\gamma_0$. The condensate field $\psi$ is initialized in a random state, but the evolution is then fully deterministic (since the noise is set to zero). The reservoir follows instantaneously the condensate dynamics. Between $t = 0$ and $t \sim 10\ \tau_p$, we observe the nucleation and exponential growing of density defects. In this regime the system can be described by linearized equations, thus the linear analysis discussed in section I B can serve as a guide to understand the time and length scales of the defect formation. The excitation spectrum (see e.g. Fig. 3a of the article) takes its maximum positive imaginary part $\mathrm{Im}[\omega_{\rm max}]$ at a wavevector $k_{\rm max} = 1/\xi_{\rm eff}$, where $\xi_{\rm eff}$ is an effective healing length [8–10] governed by the effective interaction constant $g_{\rm eff}$ (Eq. 3 of the article):

$$\xi_{\rm eff} = \frac{\hbar}{\sqrt{2m\,|g_{\rm eff}|\,\frac{\gamma_R}{R}\left(\frac{P}{P_{th}} - 1\right)}} \tag{S11}$$

The typical spacing between defects is $2\pi\xi_{\rm eff}$, while the time to develop the first density defect is of the order of $1/\mathrm{Im}[\omega_{max}]$.

Figure S2c,d shows simulations performed with the same system parameters, but without making the adiabatic approximation, i.e. by using the coupled Eqs. (1)-(2). Here, the time evolution of the reservoir is limited by the exciton loss rate ($\gamma_R \sim 10^{-2}\,\gamma_0$). This slows down the instability dynamics as compared to the adiabatic approximation. Despite quantitative differences with the adiabatic approximation, the dynamics of the instability in this two-equation model is qualitatively identical, with the chaotic propagation of density fluctuations that spoils the spatio-temporal coherence of the condensate.

Finally, for comparison we show in Fig. S2e,f simulations performed in the two-equation model but without reservoir-induced blueshift ($g_R = 0$): here, the source of the modulational instability

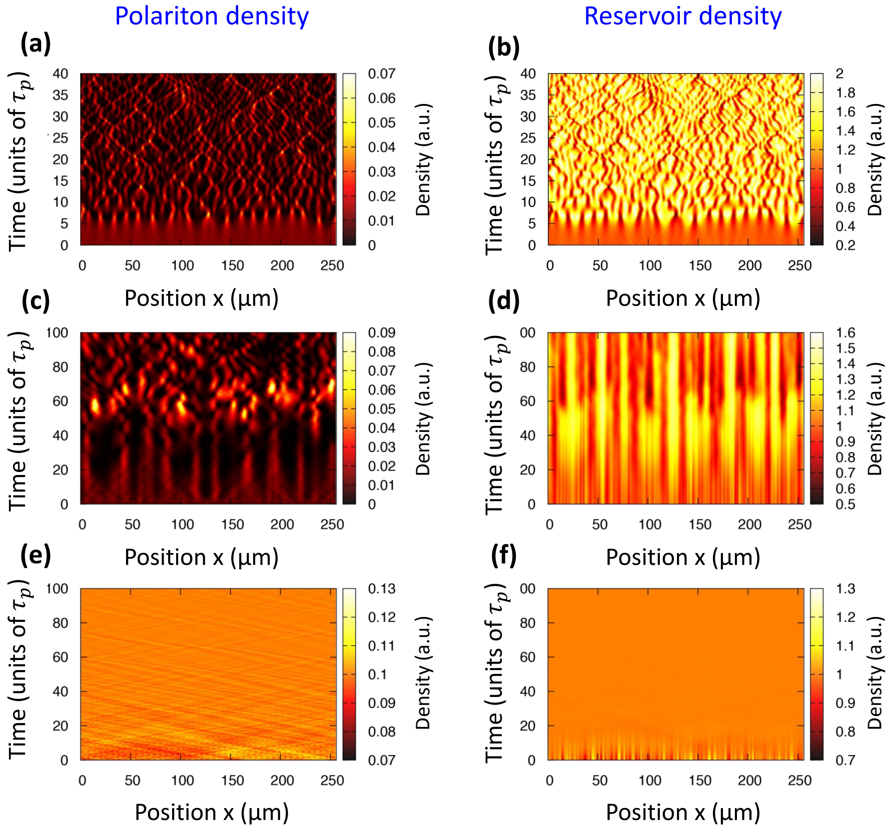


FIG. S2. Simulated time evolution of the polariton density (left column) and reservoir density (right column) for three cases: the unstable regime in the adiabatic approximation (first line), the unstable regime in the two-equation model (second line), and the stable regime in the two-equation model but without reservoir-induced blueshift (third line).

disappears and the initial perturbed state progressively relaxes to the homogeneous stable steady state.

### D. Relation between coherence time and polariton decay rate

The linear stability analysis presented above can be used to obtain a simple estimate of the coherence time in the unstable regime. For this we consider the maximum value taken by the imaginary part of the Bogoliubov spectrum, which sets the timescale of the instability:

$$\tau_{\text{instab}} = 1/\text{Im}[\omega_{max}] = \frac{\hbar}{\sqrt{\frac{\hbar^2\Gamma^2}{4} + \mu_b^2} - \frac{\hbar\Gamma}{2}} \tag{S12}$$

where $\mu_b = g_{\text{eff}}\, n_0 = g_{\text{eff}} \frac{\gamma_R}{R}\left(\frac{P}{P_{\text{th}}} - 1\right)$ and $\Gamma = \gamma\left(1 - \frac{P_{\text{th}}}{P}\right)$.

Indeed, the unstable phase dynamics of the homogeneous adiabatic condensate is described by the Kuramoto-Sivashinsky equation [7]. The chaotic properties of this equation can be mapped on the stochastic Kardar-Parisi-Zhang equation [7, 8], yielding a coherence time of the form of Eq. (S12).

Fig. S3 shows the calculation of $\tau_{\text{instab}}$ as a function of the polariton decay rate $\gamma$ using the

parameters of the main text ($P = 2\,P_{\rm th}$). Within this simplified picture which neglects localization effects induced by disorder, $\tau_{\rm instab}$, and thus the expected coherence time decreases as the polariton decay rate increases. Our experimental results and more complete numerical simulations comparing the temporal coherence of moderate and high Q cavities in Fig. 1 (l,m) of the manuscript are in agreement with this feature.

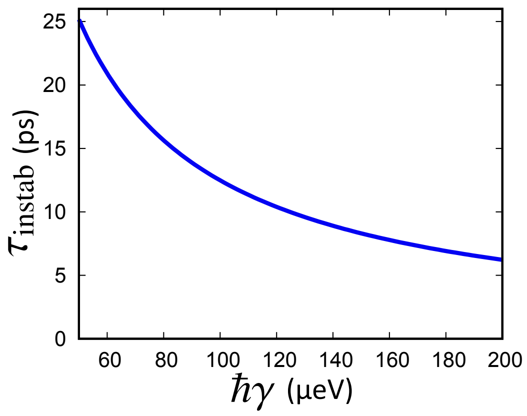


FIG. S3. Estimated coherence time in the unstable regime as a function of the polariton decay rate.

### E. Effect of disorder on the coherence properties

For simulating the different situations studied in the paper (wire cavity at moderate and high Q, and lattice) we used different numerical disorder realizations drawn from the same statistical distribution. Indeed, experimentally the disorder is different in each of the microcavity samples, and we have no direct access to it. As stated in the manuscript, we thus used the experimentally measured density profile of the condensate to infer the general shape of the disorder in each experiment, and then used this disorder profile to compute the spatiotemporal coherence.

This allowed us to show that, besides the linear stability analysis that yields the main proof of the transition from unstable to stable condensate, the shape of the density and spatiotemporal coherence altogether could also be accurately reproduced using similar disorder realizations all drawn from the same statistical distribution.

The quantitative details of the density and coherence profile depend on the detailed shape of the disorder. However we verified, both numerically and experimentally, the robustness of the qualitative features evidenced in the paper as the disorder profile is varied, i.e. sizable density inhomogeneity and low spatiotemporal coherence for positive mass condensates, versus regular density and high coherence in negative mass condensates.

As an example, Fig. S4 compares the spatial coherence of the negative mass condensate in the Lieb lattice calculated for three different disorder realizations. The blue curve corresponds to the data currently shown in Fig. 2g of the manuscript, while the orange and green curves were calculated using the disorder profile of the moderate and high Q wire cavity, used in Figs. 1g and 1k of the paper respectively. In the latter cases, we sampled the continuous disorder to map it on the discrete tight-binding model used to calculate the coherence in the lattice. We observe that the precise shape

and extension of the spatial coherence vary with the disorder potential but the qualitative trend of high coherence for negative mass condensates, signature of a stable regime, is fully preserved.

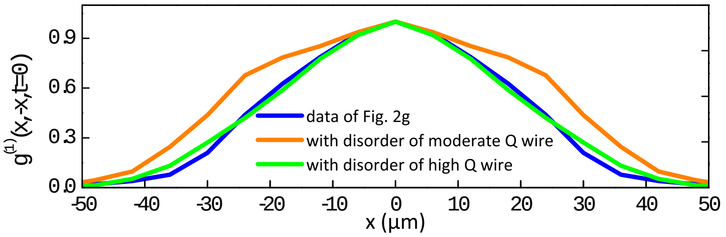


FIG. S4. Spatial coherence of the negative mass condensate in the Lieb lattice calculated for three different disorder realizations.

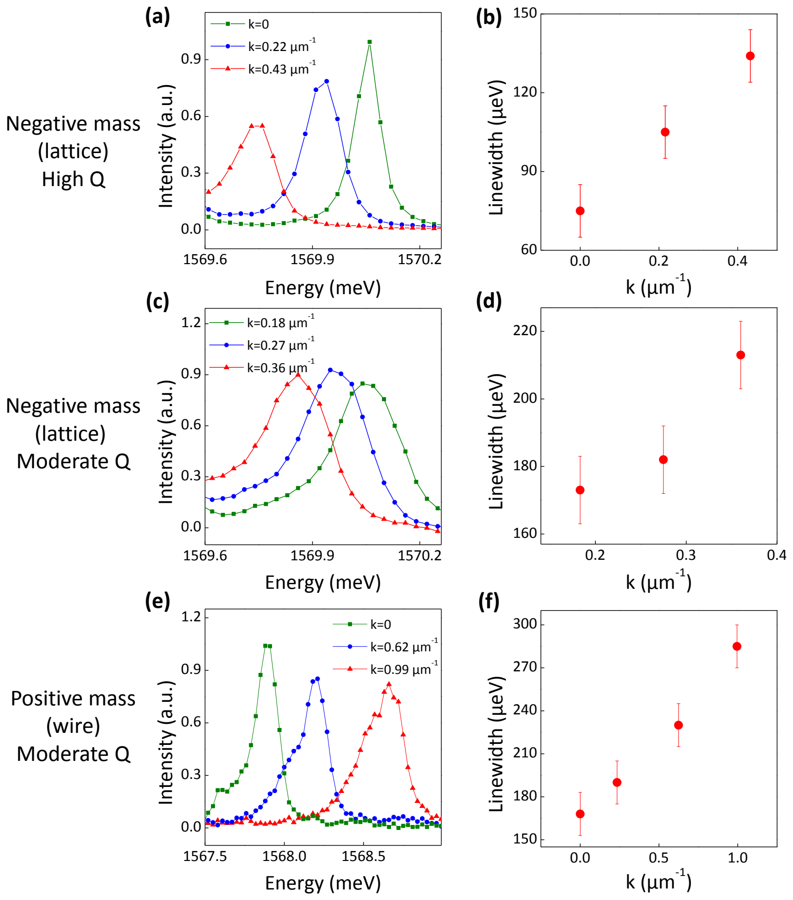


FIG. S5. (a) Low-power photoluminescence spectra for different polariton wavevectors, measured in a high $Q$ Lieb lattice. (b) Corresponding wavevector-dependence of the linewidth (as obtained from a Lorentzian fit). (c)-(d) Same measurements performed on a moderate $Q$ Lieb lattice. (e)-(f) Same measurements performed on a moderate $Q$ wire cavity.

## II. Experiment

### A. Determination of the polariton linewidth

The polariton linewidth can be estimated from the photoluminescence in the far field at very low pump power. Figure S5 shows examples of linewidth measurements for the different types of cavities studied in the article. As in the article, a polarizer is used to select the light linearly polarized along the longitudinal axis of the wire or lattice (TM polarization), which corresponds to the condensate polarization.

As mentioned in the main text, in the antisymmetric band of a lattice, the radiative linewidth is expected to increase monotonically away from the maximum of the band [3, 11]. We first checked this prediction by using a 1D Lieb lattice with high $Q$-factor and strong inter-pillar coupling (center-to-center distance of 2.4 $\mu$m), so that the three bands are well separated from each other. Figure S5a shows photoluminescence spectra of the upper band of the lattice, for different polariton wavevectors. The linewidth (FWHM) increases with $k$, as shown in Fig. S5b. The data is compatible with a linear dependence $\gamma(k) = \gamma_0 + \gamma'|k|$, with $\hbar\gamma_0 = 75\,\mu$eV and $\gamma' = 135\,\mu$eV.$\mu$m. The $k = 0$ value ($\hbar\gamma_0 = 75\,\mu$eV) appears quite high given the nominal $Q$ factor, most probably for the two following reasons. First, the emission from the whole pumped region (90 $\mu$m) is here collected, so that the linewidth is inhomogeneously broadened by disorder (typically 30 $\mu$eV). Second, electrostatic fluctuations during the integration time (about 1 second) can cause spectral wandering of the emission energy, as observed in III-V quantum dots [12]. A more precise measurement of the linewidth is usually obtained using resonant spectroscopy (in transmission) [13], but this method is not directly applicable to the samples studied here (removal of the substrate would be required). We thus used the raw experimental values given by the photoluminescence measurements.

Figures S5c-d show similar linewidth measurements carried out in a moderate $Q$ lattice. An increase of the linewidth with $k$ is also observed, with a similar rate.

Finally, Figs. S5e-f present linewidth measurements performed in a moderate $Q$ wire cavity. An increase with $k$ is also observed, albeit with a smaller slope $\gamma'/\gamma_0 \simeq 0.7\ \mu$m. Such momentum-broadening could be linked to energy relaxation, or position-dependent losses due to disorder. For completeness, we decided to include this momentum-dependence of the linewidth in the numerical simulations of the positive mass condensates: as shown in the article, this leaves the results qualitatively unchanged, and the condensate remains in the unstable regime.

### B. Spatio-temporal behavior of the coherence

The main signatures of polariton instability are given by the short spatial and temporal coherence and the density inhomogeneity (Fig. 1 of the main text) — as opposed to the smooth and highly coherent condensates obtained in the stable regime (Fig. 2). Here, we show that at moderate $Q$ factor an additional signature of the unstable regime can be obtained, by analyzing the time evolution of the spatial coherence.

Figure S6a shows the evolution of the spatial coherence profile of the moderate $Q$ wire cavity (same data set than in Fig. 1f,l of the article) when scanning the temporal delay $t$ of the interferometer. We

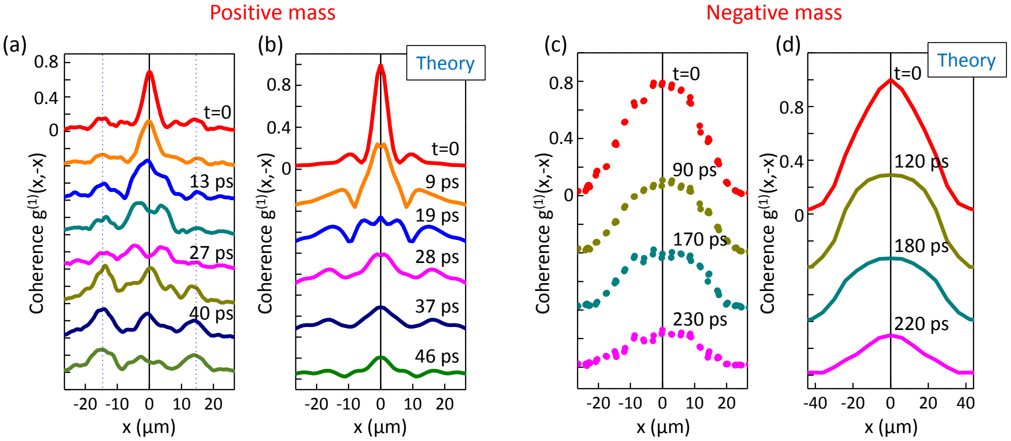


FIG. S6. (a) Measured and (b) calculated spatial coherence for different time delays $t$, in a moderate $Q$ wire cavity. (c)-(d) Same as (a) and (b), obtained in a moderate $Q$ Lieb lattice.

observe that the behavior of $g^{(1)}(x,t)$ is non-monotonic and shows a spatial spreading with time. As the time delay increases, the initial single lobe of spatial coherence splits into several lobes, so that $g^{(1)}$ becomes non-monotonic in space. $g^{(1)}(x,t)$ is also non-monotonic in time: e.g. at $x = \pm 14$ $\mu$m (indicated by vertical dotted lines) the coherence increases with time, while at $x = 0$, the coherence first decays and then regrows with time after $t = 27$ ps. This oscillatory behavior of the temporal coherence is clearly seen in Fig. 1l (green line) of the main text.

As stated in the article, this behavior can be intuitively understood from the interplay between instability and disorder: at moderate $Q$, density fluctuations chaotically propagate along the condensate, and can scatter back and forth on disorder to give rise to a non-monotonic spatio-temporal behavior of the coherence. This effect can be qualitatively reproduced by our simulations, as seen in Fig. S6b (using the same parameters than for the calculations of Fig. 1).

In the stable regime on the contrary, the evolution of the coherence is expected to be monotonic in space and time. This is confirmed in the experimental data of Fig. S6c, showing the temporal evolution of the spatial coherence profile in the 1D Lieb lattice (same data set than in Fig. 2 of the article), and in the numerical simulations of Fig. S6d (same parameters than for the calculations of Fig. 2).

---


[1] R. Huang, F. Tassone, and Y. Yamamoto, Phys. Rev. B **61**, R7854 (2000).

[2] D. Tanese, H. Flayac, D. Solnyshkov, A. Amo, A. Lemaitre, E. Galopin, R. Braive, P. Senellart, I. Sagnes, G. Malpuech, and J. Bloch, Nature Communications **4**, 1749 (2013).

[3] P. Stepnicki and M. Matuszewski, Phys. Rev. A **88**, 033626 (2013).

[4] F. Baboux, L. Ge, T. Jacqmin, M. Biondi, E. Galopin, A. Lemaître, L. Le Gratiet, I. Sagnes, S. Schmidt, H. E. Türeci, A. Amo, and J. Bloch, Phys. Rev. Lett. **116**, 066402 (2016).

[5] M. Wouters and I. Carusotto, Phys. Rev. Lett. **99**, 140402 (2007).

[6] N. Bobrovska, E. A. Ostrovskaya, and M. Matuszewski, Phys. Rev. B **90**, 205304 (2014).

[7] V. N. Gladilin, K. Ji, and M. Wouters, Phys. Rev. A **90**, 023615 (2014).

[8] P. Hohenberg and A. Krekhov, Physics Reports **572**, 1 (2015).

[9] I. S. Aranson and L. Kramer, Reviews of Modern Physics **74**, 99 (2002).

[10] L. M. Pismen, *Patterns and interfaces in dissipative dynamics* (Springer Science & Business Media, 2006).

[11] I. L. Aleiner, B. L. Altshuler, and Y. G. Rubo, Phys. Rev. B **85**, 121301 (2012).

[12] A. V. Kuhlmann, J. Houel, A. Ludwig, L. Greuter, D. Reuter, A. D. Wieck, M. Poggio, and R. J. Warburton, Nature Physics **9**, 570 (2013).

[13] S. Rodriguez, A. Amo, I. Sagnes, L. Le Gratiet, E. Galopin, A. Lemaitre, and J. Bloch, Nature communications **7** (2016).
